# Supplementary material for: Vortex Dynamics Driven Transverse Transport in Superconducting Thin Films
Source: arXiv:2605.02677 source file (2026-10-27)
Supplement: Supplementary file 1 [file 02_SI.tex]

\documentclass[aps,prl,preprint,bibliography,superscriptaddress]{revtex4-1}
\usepackage{mathrsfs}
\usepackage{amsmath,gensymb}
\DeclareMathOperator{\sign}{sign}
\usepackage{amsfonts}
\usepackage{amssymb}
\usepackage{ragged2e} 
\usepackage{amsthm}
\usepackage{graphicx}
\usepackage{natbib}
\usepackage{color}
\usepackage{hyperref}
\usepackage{bm}
\usepackage[caption=false]{subfig}
\usepackage{caption}

\setcounter{figure}{0}

\usepackage{verbatim}

\setcounter{secnumdepth}{3}

\begin{document}
\title{Supporting information for the article \\Vortex Transport in Ni/Bi Bilayer Superconductor with Strong Spin-Orbit and Exchange Interaction}
\author{Laxmipriya Nanda}
\affiliation{Centre for Nanoscience and Engineering, Indian Institute of Science, Bengaluru, Karnataka 560012, India} 
\author{Sohini Guin}
\affiliation{Centre for Nanoscience and Engineering, Indian Institute of Science, Bengaluru, Karnataka 560012, India} 
\author{Yasen Hou}
\affiliation{Plasma Science and Fusion Center, Massachusetts Institute of Technology, Cambridge 02139, USA} 
\author{Rajib Sarkar}
\affiliation{Centre for Nanoscience and Engineering, Indian Institute of Science, Bengaluru, Karnataka 560012, India} 
\author{Naresh Shyaga}
\affiliation{Centre for Nanoscience and Engineering, Indian Institute of Science, Bengaluru, Karnataka 560012, India} 
\author{Souvik Banerjee}
\affiliation{Jawaharlal Nehru Center for Advanced Scientific Research, Jakkur, Bengaluru}
\author{A. Sundaresan}
\affiliation{Jawaharlal Nehru Center for Advanced Scientific Research, Jakkur, Bengaluru}
\author{N. S. Vidhyadhiraja}
\affiliation{Jawaharlal Nehru Center for Advanced Scientific Research, Jakkur, Bengaluru}
\author{Jagadeesh S. Moodera}
\affiliation{Plasma Science and Fusion Center, Massachusetts Institute of Technology, Cambridge 02139, USA} 
\affiliation{Department of Physics, Massachusetts Institute of Technology, Cambridge 02139, USA} 
\author{Dhavala Suri}
\email{dsuri@iisc.ac.in}
\affiliation{Centre for Nanoscience and Engineering, Indian Institute of Science, Bengaluru, Karnataka 560012, India} 
\maketitle

\section{HRTEM data}
\begin{figure}[h]
    \centering
    \includegraphics[width=0.9\textwidth]{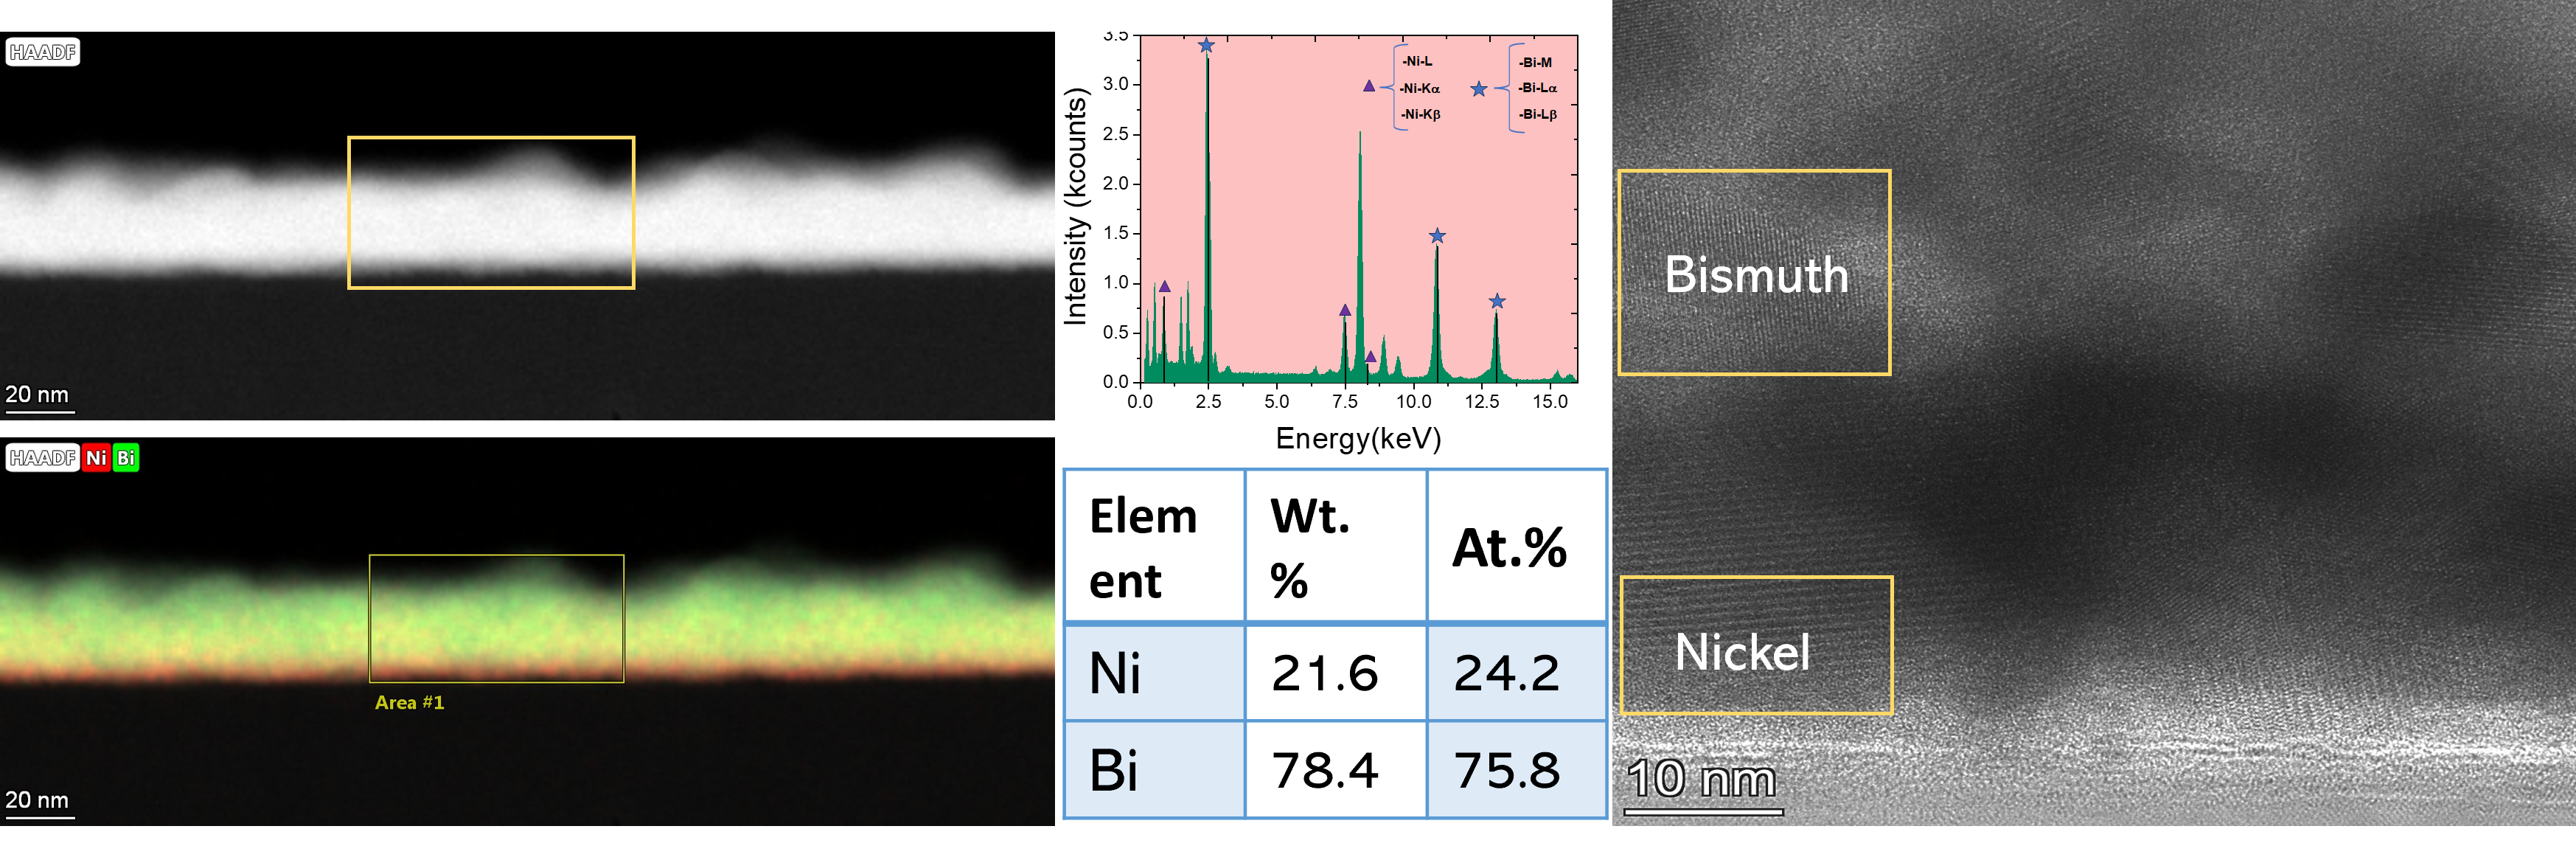}
    \caption{EDAX mapping and HRTEM of Ni/Bi sample}
\label{fig-S1}
\end{figure}
\section{Transport characteristics}
A series of transport measurements were carried out on Ni/Bi and Ni/Bi/EuS samples to examine the reproducibility of the observed features. The corresponding background study data are provided in this section.
Figure-S2, shows the evident feature of Tc vs B analysis for both NiBi and NiBiEuS sample. Figure-S2(a) represents the Tc vs B for Ni/Bi bilayer sample showing the 2D to 3D-GL crossover. The formula used for fitting the two different regions are shown in Equation-S1 and S2. 

\begin{figure}[h]
    \centering
    \includegraphics[width=0.9\textwidth]{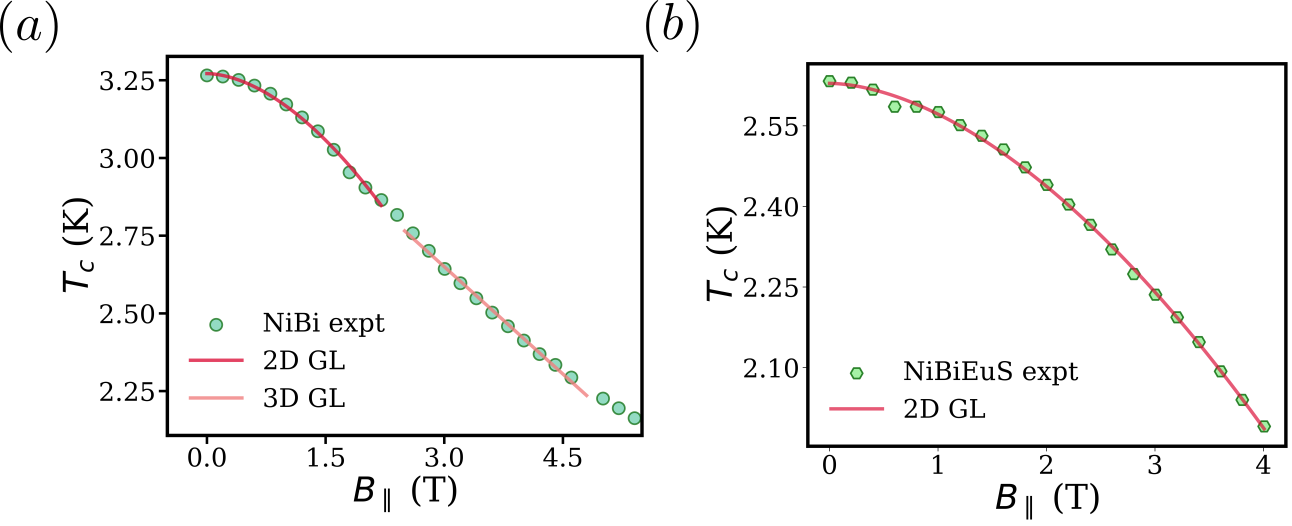}
    \caption{(a) Tc vs B for NiBi sample showing 2D to 3D crossover (b) Tc vs B for NiBiEus sample data fitted with 2D-GL model}
\label{fig-S2}
\end{figure}

The 2D-GL model which is being used here to fit our experimental curve:
\begin{equation}
T_c(B) = T_{c0}\left[1 - \left(\frac{B}{B_c}\right)^n \right],
\tag{S1}
\end{equation}
where n=2 is the best fitting of the data. 

Similarly the 3D-GL model used for fitting of NiBi experimental data in the range of 2.5T to 4.5T is:
\begin{equation}
T_c(B) = T_{c0}\left(1 - \frac{B}{B_c}\right)
\tag{S2}
\end{equation}

\begin{figure}
    \centering
    \includegraphics[width=0.7\linewidth]{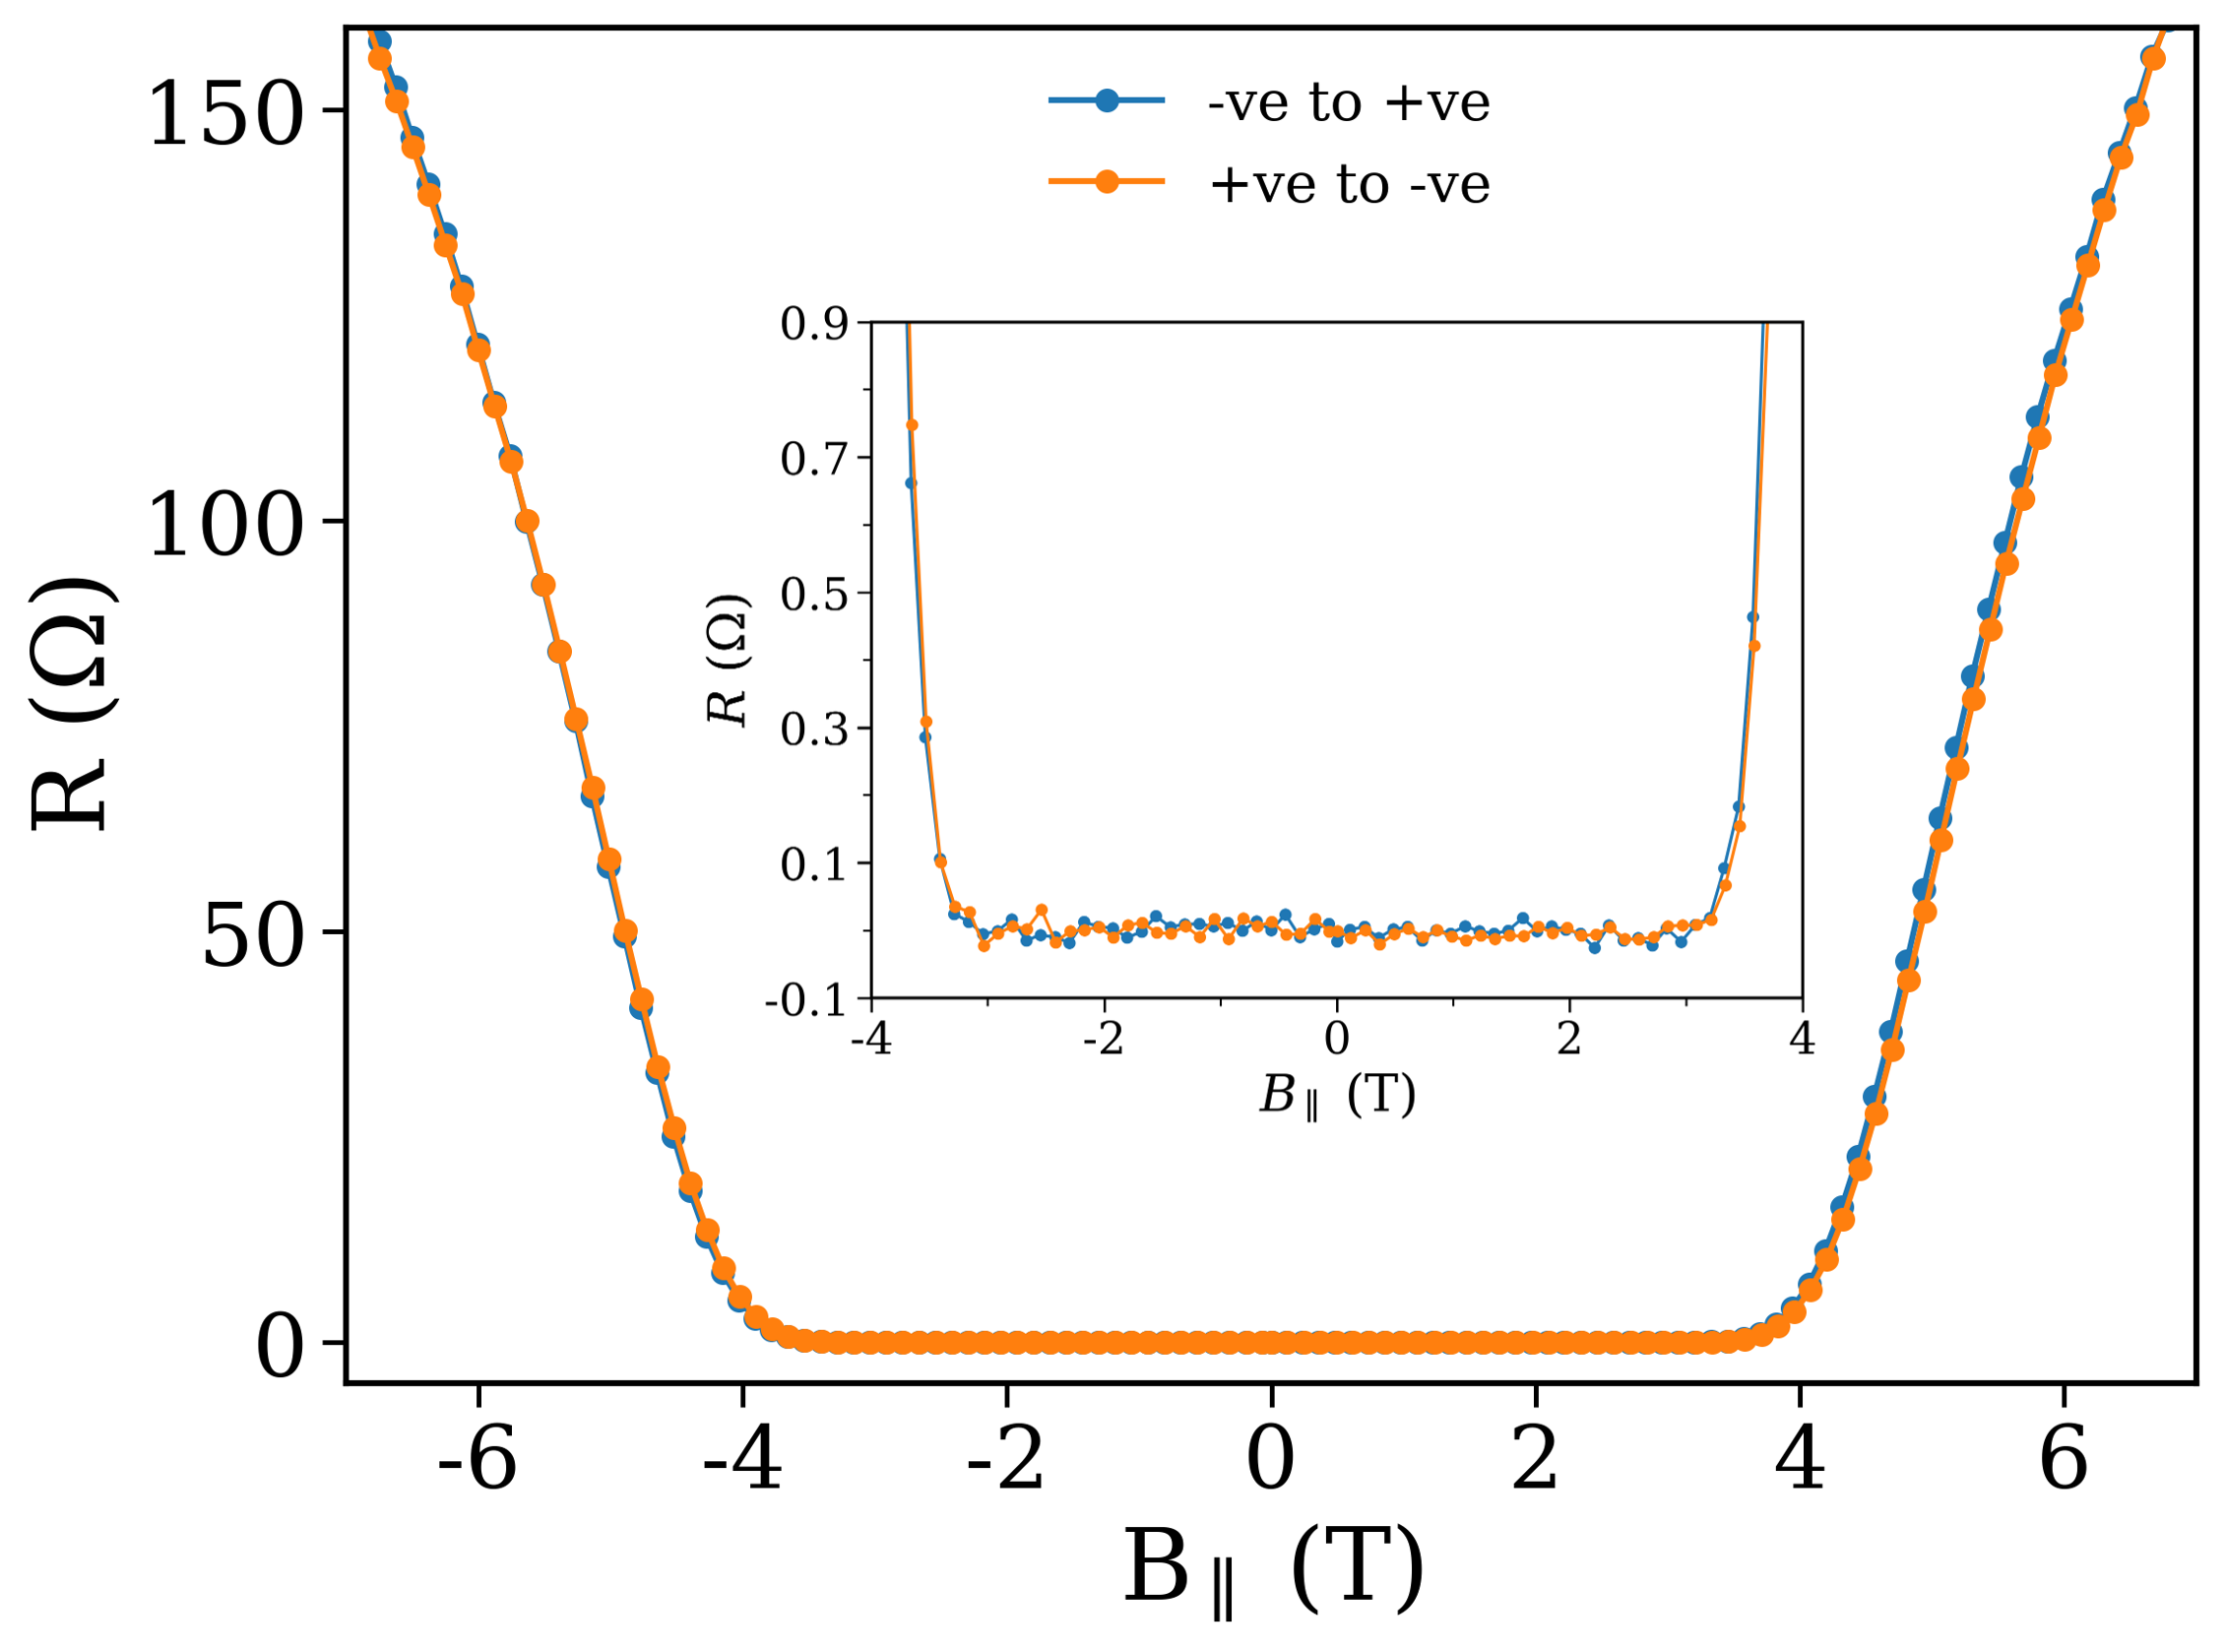}
\caption{Resistance vs magnetic field (B$_\parallel$) for Ni/Bi bilayer sample. Inset: Zoomed region showing no hysteresis.}
\label{fig:S2}
\end{figure}
Figure-S3 represents Resistance vs magnetic field for Ni/Bi bilayer sample where the hysteresis is not present. 

\section{Magnetisation of Ni/Bi/EuS sample}
\begin{figure}[h]
    \centering
    \includegraphics[width=0.9\textwidth]{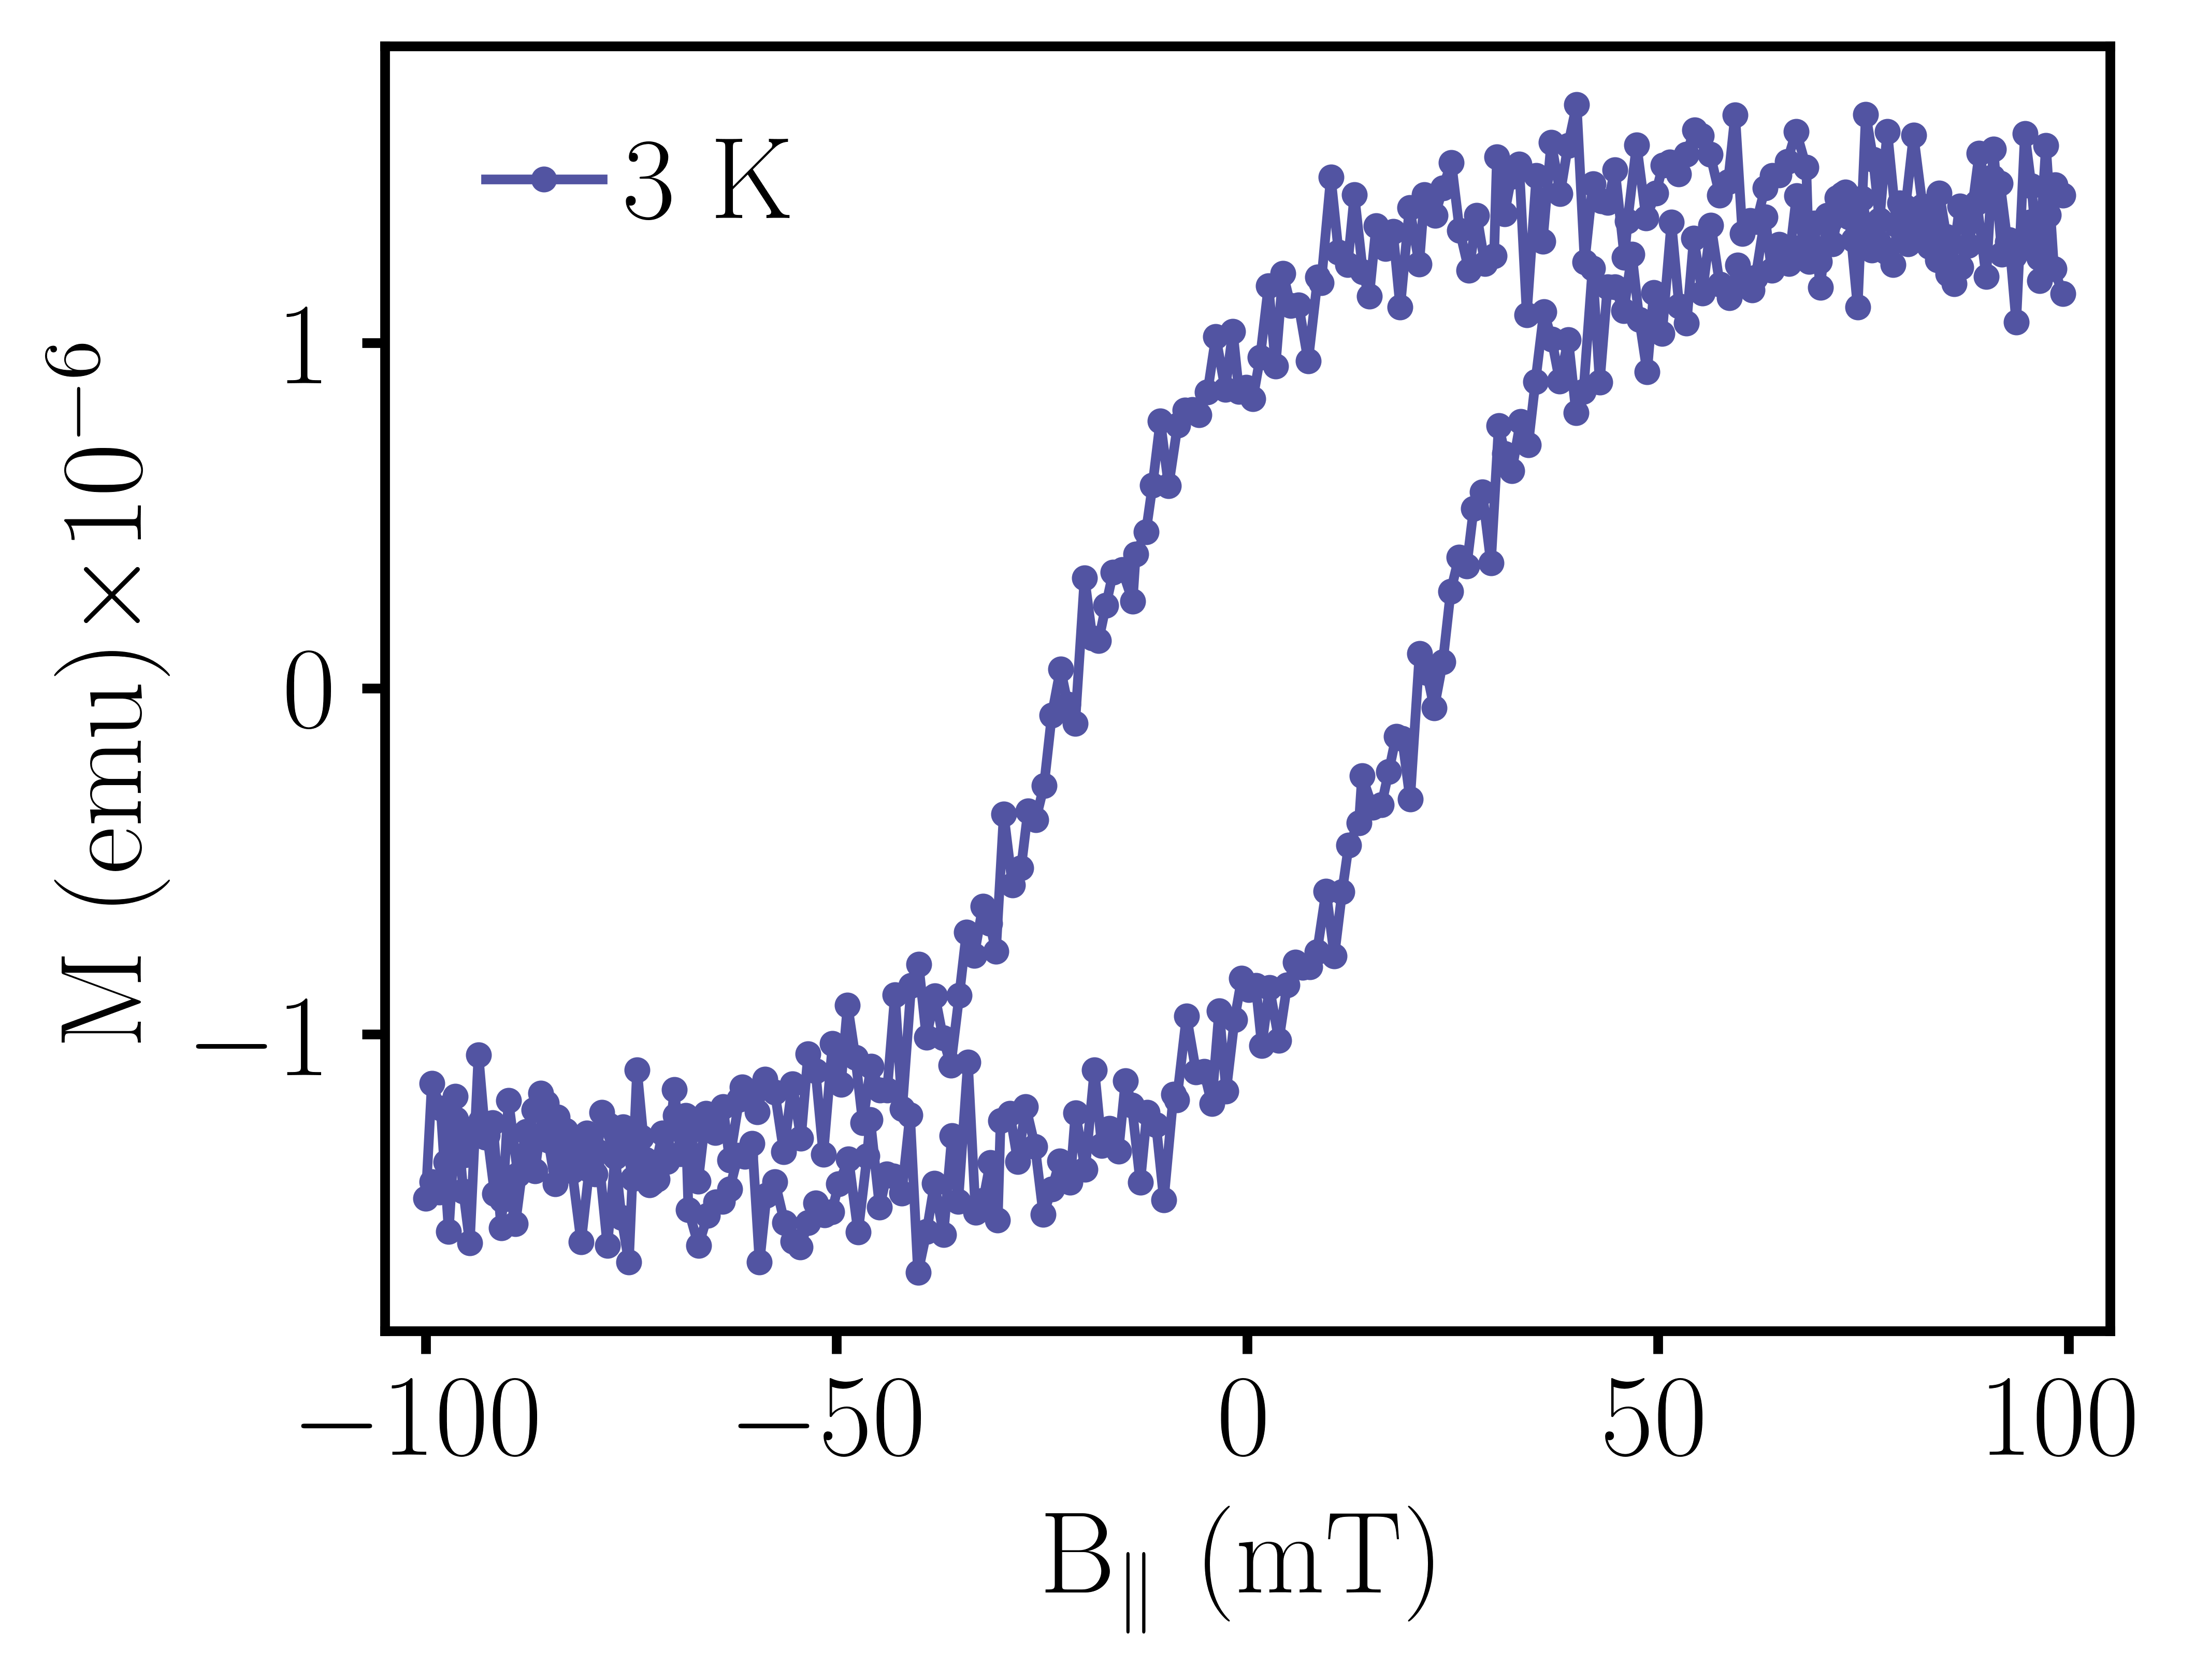}
    \caption{Magnetization versus applied field of the Ni/Bi/EuS sample at 3 K}
\label{fig-S1}
\end{figure}

The coercive field of the hetero-structure stack is $\approx$ 10 mT which is comparable with the field at which the $T_c$ of the stack. This indicates that the magnetization of the sample and the measured peak in $T_c$ are correlated. The non-square hysteresis loop indicates that magnetization reversal is not coherent but occurs via multi-step or domain-driven processes. In our Ni/Bi/EuS hetero-structure, this likely arises from the coexistence of two ferromagnetic layers with different coercivities and anisotropies, along with weak interlayer coupling and interface-induced magnetic disorder. This leads to a gradual switching behavior and reduced remanence. 

\section{Field-Dependence of the viscous drag and the Hall parameter}

The equation of motion derived for a single vortex from a balance of forces is found to be:
\begin{equation}
\eta \bm{v}_L + \alpha_H \left(\bm{v}_L \times \hat{\bm{k}} \right) = \bm{F}_L .
\end{equation}

As discussed in the main manuscript, the present equation of motion does not explicitly account for pinning effects or vortex–vortex interactions. While these contributions are known to play a significant role, particularly in the mixed state, their rigorous incorporation requires a detailed and system-specific treatment of vortex dynamics, which lies beyond the scope of the present work. Accordingly, these effects are included here in an effective, phenomenological manner through an explicit field ($H$) dependence of the parameters, $\eta$ and $\alpha_H$, as described below:
\begin{align}
    \eta(H) & = \epsilon_0 H_2\left(1+\epsilon_1\frac{|B|}{H_2}\right) \\
    \alpha_H(H) & =\alpha_0\frac{B}{H_2} \left( 1- \frac{|B|}{H_2}\right) \theta(H_2-|B|)
\end{align}
where $B=\xi H_2 \,u\,\theta(u),\, \xi=\sign(H)$, and $u=\frac{|H| - H_1}{H_2-H_1}$. The initial guess for the parameters, $H_1$ and $H_2$ is found by observing where $\rho_{xx}$ rises from zero, and saturates, respectively. The table below lists the values of the parameters, $\{\alpha_0, \epsilon_0, \epsilon_1, H_1, H_2\}$, obtained by fitting theory to experiments.

% @Rajib, please add the table of the best fit parameters here.

\begin{tabular}{|p{2.5cm}|p{1.8cm}|p{1.8cm}|p{1.5cm}|p{2cm}|p{2.5cm}|}
\hline
\textbf{T (K)} & \boldmath$\alpha$ & \boldmath$\epsilon_{0}$ & \boldmath$\epsilon_{1}$ & \textbf{H$_{1}$} & \textbf{H$_{2}$} \\
\hline
2.3 & -1.40  & 0.6129 & 2.29 & 1.802 & 2.373 \\
3.2 & -0.841 & 0.1473 & 4.77 & 0.925 & 1.28 \\
3.6 & -1.20 & 0.156 & 5.06 & 0.36 & 0.707 \\
\hline
\end{tabular}

\end{document}
